# Supplementary material for: Passport: Enabling Accurate Country-Level Router Geolocation using Inaccurate Sources
Source: arXiv:1905.04651 source file (2019-07-23)
Supplement: Supplementary file 1 [file geoloc-appendix.tex]

\cleardoublepage
\section*{\\Appendix}

%\appendix
\subsection{\\Title of Appendix A}
% the \\ insures the section title is centered below the phrase: AppendixA

Text of Appendix A is Here

\section{\\Title of Appendix B}
% the \\ insures the section title is centered below the phrase: Appendix B

Text of Appendix B is Here
